# Supplementary material for: Enhancing Product Safety in E-Commerce with NLP
Source: arXiv:2210.14363 source file (2022-10-25)
Supplement: Supplementary file 1 [file appendix.tex]

%This step requires \textit{one time} human supervision to interpret numeric ratings 
%into `natural language'.
% TREC taxonomy: https://cogcomp.seas.upenn.edu/Data/QA/QC/definition.html
\begin{table}[h]
\centering
\resizebox{0.7\textwidth}{!}{%
\begin{tabular}{ccc}
\hline
Rating & ${\textsc{Amazon}}_{\textsc{full}}$ & Yelp-full \\ \hline
1 & very negative product sentiment & very negative restaurant sentiment \\
2 & negative product sentiment & negative restaurant sentiment \\ 
3 & neutral product sentiment & neutral restaurant sentiment \\ 
4 & positive product sentiment & positive restaurant sentiment \\ 
5 & very positive product sentiment & very positive restaurant sentiment \\ \hline
\end{tabular}%
}
\caption{Interpretation of numeric ratings in `natural language', used by TARS.}
\label{tab:}
\end{table}

\subsection{Experimental Setup}
\label{subsec:experimental_setup}
